# Supplementary material for: Dislocation defect as a bulk probe of monopole charge of multi-Weyl semimetals
Source: arXiv:1911.11146 ancillary file (2020-02-21)
Supplement: Supplementary file 1 [file SM-Final.pdf]

# Supplemental Material for "Dislocation defect as a bulk probe of monopole charge of multi-Weyl semimetals

Rodrigo Soto-Garrido,[1] Enrique Muñoz,[1] and Vladimir Juričić[2]

[1] *Facultad de Física, Pontificia Universidad Católica de Chile, Vicuña Mackenna 4860, Santiago, Chile*
[2] *Nordita, KTH Royal Institute of Technology and Stockholm University, Roslagstullsbacken 23, 10691 Stockholm, Sweden*

(Dated: January 28, 2020)

## CONTENTS

S1. Landau levels of multi-Weyl semimetal 1
A. Angular momentum 3
B. Wavefunctions in real space 3
1. Wavefunction of the lowest Landau level (LLL) 4

S2. Scattering analysis 4

S3. Transmission and Landauer conductance 7

S4. Dimensionless quantities 9

S5. Normalization constants 9

References 10

## S1. LANDAU LEVELS OF MULTI-WEYL SEMIMETAL

In this section we provide the details of the calculation of the Landau levels of a multi-Weyl semimetal featuring two nodal points with the monopole charge $\xi n$, with $\xi = \pm$ as the nodal (valley) index, and $n > 0$. We consider the continuum Hamiltonian in momentum space describing non-interacting low-energy nodal quasiparticles (Eq. (1) of the main text)

$$H_\xi^{(n)} = \begin{pmatrix} \xi v_z k_z & \alpha_n (k_x - i k_y)^n \\ \alpha_n (k_x + i k_y)^n & -\xi v_z k_z \end{pmatrix}. \tag{S1}$$

As detailed in the main text of the paper, the effect of the screw dislocation on the gapless quasiparticles is described by a constant pseudo-magnetic field confined within its core, whose sign depends on the node signature, i.e. $\xi \mathbf{B}_D$, with $\mathbf{B}_D = B_D \mathbf{e}_z$. This pseudo-magnetic field is included in the effective Hamiltonian by minimal (Peierls) substitution ($e = \hbar = k_B = 1$ hereafter):

$$\boldsymbol{k} \to \boldsymbol{k} + \xi \boldsymbol{A}_D \equiv \boldsymbol{\Pi}^\xi. \tag{S2}$$

It is then straightforward to show that

$$[\Pi_x^\xi, \Pi_y^\xi] = -i\xi B_D = -i\xi \ell^{-2}, \tag{S3}$$

where $\ell = 1/\sqrt{B_D}$ is the magnetic length. In addition, it is convenient to define the lowering and raising operators as $a = \ell\left(\Pi_x^\xi - i\xi\Pi_y^\xi\right)/\sqrt{2}$ and $a^\dagger = \ell\left(\Pi_x^\xi + i\xi\Pi_y^\xi\right)/\sqrt{2}$, respectively, obeying the canonical commutation relation $[a, a^\dagger] = 1$. Using this definition, we write the effective Hamiltonian in the vicinity of each of the two nodes at $\xi = \pm$ as

$$H_\xi^{(n)} = \begin{pmatrix} \xi v_z k_z & \alpha_n \left(\frac{\sqrt{2}}{\ell} a\right)^n \\ \alpha_n \left(\frac{\sqrt{2}}{\ell} a^\dagger\right)^n & -\xi v_z k_z \end{pmatrix}. \tag{S4}$$

The above Hamiltonian can be diagonalized in terms of the number states $\{|m\rangle\}$, satisfying the ladder equations $a|m\rangle = \sqrt{m}|m-1\rangle$ and $a^\dagger|m\rangle = \sqrt{m+1}|m+1\rangle$, with $m \geq 0$ and $a|0\rangle = 0$. The Landau levels (LLs) for each node then satisfy

$$H_\xi^{(n)}|\Psi_m^{(\lambda,\xi)}\rangle = \lambda E_m^\xi|\Psi_m^{(\lambda,\xi)}\rangle. \tag{S5}$$

We point out that the effective Hamiltonians at the two nodes are related by a similarity (unitary) transformation

$$H_-^{(n)} = \sigma_x\, H_+^{(n)}\sigma_x, \tag{S6}$$

and the spectrum of both operators is therefore exactly the same. More explicitly,

$$\begin{pmatrix} \xi v_z k_z & \alpha_n\left(\frac{\sqrt{2}}{\ell}a\right)^n \\ \alpha_n\left(\frac{\sqrt{2}}{\ell}a^\dagger\right)^n & -\xi v_z k_z \end{pmatrix}\begin{pmatrix} |u_m\rangle \\ |v_m\rangle \end{pmatrix} = \lambda E_m \begin{pmatrix} |u_m\rangle \\ |v_m\rangle \end{pmatrix}, \tag{S7}$$

leading to the following system of coupled equations

$$\alpha_n\left(\frac{\sqrt{2}}{\ell}\right)^n a^n|v_m\rangle = \left(\lambda E_m - \xi v_z k_z\right)|u_m\rangle \tag{S8}$$

$$\alpha_n\left(\frac{\sqrt{2}}{\ell}\right)^n (a^\dagger)^n|u_m\rangle = \left(\lambda E_m + \xi v_z k_z\right)|v_m\rangle. \tag{S9}$$

By combining Eqs. (S8) and (S9), we obtain

$$\left(\frac{2}{\ell^2}\right)^n \alpha_n^2 (a^\dagger)^n a^n|v_m\rangle = \left(E_m^2 - \xi^2 v_z^2 k_z^2\right)|v_m\rangle. \tag{S10}$$

Finally, using the properties of the raising and lowering operators (trivially demonstrated by induction)

$$\begin{aligned} a^n|m\rangle &= \sqrt{m(m-1)(m-2)\ldots(m-n+1)}|m-n\rangle \\ (a^\dagger)^n|m\rangle &= \sqrt{(m+1)(m+2)\ldots(m+n)}|m+n\rangle, \end{aligned} \tag{S11}$$

we find that

$$(a^\dagger)^n a^n|m\rangle = \frac{m!}{(m-n)!}|m\rangle, \quad m \geq n, \tag{S12}$$

with the corresponding expression for the energy of the LLs

$$E_m = \sqrt{(v_z k_z)^2 + \left(\frac{2\alpha_n^{2/n}}{\ell^2}\right)^n \frac{m!}{(m-n)!}}, \tag{S13}$$

and $\lambda = \pm$ representing the two bands $\lambda E_m$, $m \geq n$. The corresponding eigenstates are thus given by the following spinor:

$$|\Psi_m^{(\lambda,\xi)}\rangle = \mathcal{C}\begin{pmatrix} \chi_+|m-n\rangle \\ \lambda\chi_-|m\rangle \end{pmatrix}, \tag{S14}$$

with $\chi_\mu \equiv \chi_\mu(\lambda, \xi = +, v_z, k_z, E_m) = \sqrt{1 + \mu\lambda(v_z k_z/E_m)}$, and $\mu = \pm$, while $\mathcal{C}$ an overall normalization constant (see Sec. S5). Here, the function $\chi_\mu(\lambda, \xi, v_z, k_z, E) = \sqrt{1 + \mu\lambda\xi(v_z k_z/E)}$, in general. For $m < n$ we have

$$|\Psi_m^{(\lambda,\xi)}\rangle = \begin{pmatrix} 0 \\ |m\rangle \end{pmatrix}, \tag{S15}$$

with $E_m = \lambda\xi v_z k_z$.

### A. Angular momentum

In this section we show that $[H_\xi^{(n)}, J_z] = 0$, where $J_z = L_z + nS_z$ is the total angular momentum, with $S_z = \sigma_z/2$. For this purpose is more convenient to express the Hamitonian in Eq. (S4) in terms of $\sigma_\pm = (\sigma_x \pm \sigma_y)/2$ as

$$H_\xi^{(n)} = \alpha_n \omega^n \left(a^n \sigma_+ + (a^\dagger)^n \sigma_-\right) + \xi v_z k_z \sigma_z, \tag{S16}$$

where we have defined $\omega = \sqrt{2}/\ell$. For concreteness, in the following we use the symmetric gauge $\mathbf{A}_D = (B_D/2)(-y\mathbf{e}_x + x\mathbf{e}_y)$. Using the property on equation (S6) we now focus on the case $\xi = +$ without loss of generality. In this gauge, the lowering operator can be expressed as

$$a = \frac{\ell}{\sqrt{2}}\left(k_x - \frac{y}{2\ell^2} - ik_y - i\frac{x}{2\ell^2}\right). \tag{S17}$$

Using the definition of the $z$ component of orbital angular momentum $L_z = xk_y - yk_x$ and the canonical commutation relations ($[x, k_x] = [y, k_y] = i$ and the rest of the commutators equal to zero) we obtain

$$[a, L_z] = a, \text{ and } [a^\dagger, L_z] = -a^\dagger. \tag{S18}$$

Therefore $[a^n, L_z] = na^n$, $[(a^\dagger)^n, L_z] = -n(a^\dagger)^n$ and finally

$$[H_+^{(n)}, L_z] = n\alpha_n\omega^n \left(a^n\sigma_+ - (a^\dagger)^n\sigma_-\right). \tag{S19}$$

We now compute $[H_+^{(n)}, S_z] = \frac{1}{2}[H_+^{(n)}, \sigma_z]$. Using the commutation relations of the Pauli matrices $[\sigma_k, \sigma_l] = 2i\epsilon_{klm}\sigma_m$ we have that $[\sigma_\pm, \sigma_z] = \mp 2\sigma_\pm$. We therefore find

$$[H_+^{(n)}, S_z] = \frac{1}{2}[H_+^{(n)}, \sigma_z] = \frac{1}{2}\alpha_n\omega^n \left(a^n[\sigma_+, \sigma_z] + (a^\dagger)^n[\sigma_-, \sigma_z]\right) = \alpha_n\omega^n\left(-a^n\sigma_+ + (a^\dagger)^n\sigma_-\right). \tag{S20}$$

Eqs. (S19) and (S20) then together yield

$$[H_+^{(n)}, J_z] = 0. \tag{S21}$$

### B. Wavefunctions in real space

We now compute the Landau Levels wave functions in position space. Defining $u = x/\sqrt{2}\ell$ and $u = y/\sqrt{2}\ell$ we have

$$a = -\frac{i}{2}\left[\partial_u - i\partial_v + (u - iv)\right]. \tag{S22}$$

It is convenient to work with the complex variables defined by $z = u + iv$ and $\bar{z} = u - iv$ in terms of which the dericatives read

$$\partial_z = \frac{1}{2}\left(\partial_u - i\partial_v\right) \text{ and } \partial_{\bar{z}} = \frac{1}{2}\left(\partial_u + i\partial_v\right) \tag{S23}$$

The lowering and raising operators are then represented as

$$a = -i\left[\partial_z + \frac{\bar{z}}{2}\right] \text{ and } a^\dagger = -i\left[\partial_{\bar{z}} - \frac{z}{2}\right]. \tag{S24}$$

The orbital angular momentum $L_z$ in complex coordinates is given by

$$L_z = z\partial_z - \bar{z}\partial_{\bar{z}}, \tag{S25}$$

while, in the same representation, the spinor eigenfunction in Eq. (S14) reads

$$\Psi_m^{(\lambda,\xi)}(z, \bar{z}) = \mathcal{C}\begin{pmatrix} \chi_+\psi_{m-n}(z,\bar{z}) \\ \lambda\chi_-\psi_m(z,\bar{z}) \end{pmatrix}, \tag{S26}$$

with $\psi_{m-n}(z, \bar{z}) = \langle z, \bar{z}|m\rangle$, and $\mathcal{C} = \frac{1}{\sqrt{4\pi L\ell^2(|M|+m-n/2)!}}$, which is explicitly evaluated in Sec. S5.

### 1. Wavefunction of the lowest Landau level (LLL)

To compute the wavefunction of the LLL we use that $a|0\rangle = 0$, implying

$$\left[\partial_z + \frac{\bar{z}}{2}\right]\psi_0(z,\bar{z}) = 0 \implies \psi_0(z,\bar{z}) = f(\bar{z})e^{-z\bar{z}/2} \tag{S27}$$

where $f(\bar{z})$ is an antiholomorphic function.

We now use the fact that the angular momentum commutes with the Hamiltonian in Eq. (S4) so that spinor eigenstate can be chosen to be an eigenstate of $J_z' = L_z + \frac{n}{2}\sigma_z$, i.e. $J_z'|\Psi_m^\xi\rangle = M|\Psi_m^\xi\rangle$.

$$\psi_0(z,\bar{z}) = \bar{z}^{-M\pm n/2}e^{-z\bar{z}/2} \tag{S28}$$

where the $\pm$ sign correspond to the upper and lower component of the spinor $|\Psi_m^{(\lambda,\xi)}\rangle$ in Eq. (S26).

To generate the higher Landau levels, we apply the raising operator

$$|m\rangle = \frac{1}{\sqrt{m!}}(a^\dagger)^m|0\rangle, \tag{S29}$$

which yields

$$\psi_m(z,\bar{z}) = \frac{1}{\sqrt{m!}}(-i)^m\left[\partial_{\bar{z}} - \frac{z}{2}\right]^m \bar{z}^{-M\pm n/2}e^{-z\bar{z}/2}. \tag{S30}$$

We then define $w = z\bar{z}$ to obtain

$$\left[\partial_{\bar{z}} - \frac{z}{2}\right]^m \bar{z}^{-M\pm n/2}e^{-z\bar{z}/2} = z^{m+M\pm n/2}\left(\partial_w - \frac{1}{2}\right)^m w^{-M\mp n/2}e^{-w/2} \tag{S31}$$

The right hand side of the previous equation generates the associated Laguerre polynomials [1], yielding

$$\psi_m^M(z,\bar{z}) = \sqrt{m!}(-i)^m\bar{z}^{-m-M\mp n/2}L_m^{-m-M\mp n/2}(z\bar{z})e^{-z\bar{z}/2} \tag{S32}$$

After recalling that

$$\begin{aligned} z &= u + iv = \frac{x+iy}{\sqrt{2}\ell} = \frac{r}{\sqrt{2}\ell}e^{i\phi} \\ \bar{z} &= u - iv = \frac{x-iy}{\sqrt{2}\ell} = \frac{r}{\sqrt{2}\ell}e^{-i\phi}, \end{aligned} \tag{S33}$$

we finally write the wave function in cylindrical coordinates

$$\Psi_{m,M}^{(\lambda,\xi)}(\mathbf{r}) = \frac{e^{-r_\ell^2/2}e^{ik_z z}}{\sqrt{4\pi L\ell^2(|M|+m-n/2)!}}\begin{pmatrix} \chi_+ C(m-n, r_\ell, |M|+n/2)e^{i(M-\frac{n}{2})\phi} \\ \lambda\chi_- C(m, r_\ell, |M|-n/2)e^{i(M+\frac{n}{2})\phi}\end{pmatrix}, \tag{S34}$$

where the functions $\chi_\mu \equiv \chi_\mu(\lambda, \xi = +, v_z, k_z, E_m)$ defined after Eq. (S14), $C(m, r_\ell, n) = \sqrt{m!}(-i)^m r_\ell^n L_m^n(r_\ell^2)$, with $r_\ell \equiv r/\ell\sqrt{2}$, and $L_m^n(x)$ as the associated Laguerre polynomial. This is Eq. (6) of the main text.

## S2. SCATTERING ANALYSIS

In what follows, we shall closely follow the analysis presented by some of us in Ref.[2, 3]. For this purpose, we consider an incident free-spinor propagating towards the dislocation in the $x$-direction, which is readily obtained from the free Hamiltonian in Eq. (S1)

$$\Psi_{inc}^{(\lambda,\xi)}(\mathbf{r}) = \frac{1}{\sqrt{2}}\begin{pmatrix}\chi_+ \\ \lambda\chi_-\end{pmatrix}e^{ik_\perp r\cos\phi + ik_z z}, \tag{S35}$$

where $\chi_\mu \equiv \chi_\mu(\lambda, \xi, v_z, k_z, \epsilon_{n,\boldsymbol{k}})$ defined after Eq. (S14), and the energy of the free gapless quasiparticle is

$$\epsilon_{n,\boldsymbol{k}}^\lambda = \lambda\sqrt{\alpha_n^2 k_\perp^{2n} + v_z^2 k_z^2} \equiv \lambda\epsilon_{n,\mathbf{k}}, \tag{S36}$$

with $\lambda = \pm$. Moreover, for the purposes of the scattering analysis, it is convenient to express the incident state above by using the mathematical identity

$$e^{ik_\perp r\cos\phi} = \sum_{m'\in\mathbb{Z}} i^{m'} e^{im'\phi} J_{m'}(k_\perp r), \tag{S37}$$

such that Eq.(S35) becomes

$$\Psi_{inc}^{(\lambda,\xi)}(\mathbf{r}) = \frac{e^{ik_z z}}{\sqrt{2}} \sum_{m'\in\mathbb{Z}} \begin{pmatrix} i^{m'}\chi_+ e^{im'\phi} J_{m'}(k_\perp r) \\ \lambda i^{m'}\chi_- e^{i(m'+n)\phi} J_{m'}(k_\perp r) \end{pmatrix}. \tag{S38}$$

On the other hand, the outgoing state emerging from the dislocation is given by a linear superposition of the incident and the scattered states of the form

$$\Psi_{out}^{(\lambda,\xi)}(\mathbf{r}) = \Psi_{inc}^{(\lambda,\xi)}(\mathbf{r}) + \begin{pmatrix} f_1(\phi) \\ f_2(\phi) \end{pmatrix} \frac{e^{ik_\perp r + ik_z z}}{\sqrt{r}}. \tag{S39}$$

To find the form of the phase shifts, we first asymptotically match the above form of the scattered state to the general solution for a free spinor,

$$H_\xi^{(n)} \Psi_{out}^{(\lambda,\xi)}(\mathbf{r}_\perp, z) = \lambda\epsilon_{n,\mathbf{k}} \Psi_{out}^{(\lambda,\xi)}(\mathbf{r}_\perp, z), \tag{S40}$$

where $\mathbf{r}_\perp = (x, y)$, and the Hamiltonian operator acquires the form

$$H_\xi^{(n)} = \begin{pmatrix} \xi v_z(-i\partial_z) & \alpha_n\left(-i\partial_x - i(-i\partial_y)\right)^n \\ \alpha_n\left(-i\partial_x + i(-i\partial_y)\right)^n & -\xi v_z(-i\partial_z) \end{pmatrix}. \tag{S41}$$

We write the free-spinor eigenfunction in the form

$$\Psi_{out}^{(\lambda,\xi)}(\mathbf{r}_\perp, z) = \begin{pmatrix} F(\mathbf{r}_\perp) \\ G(\mathbf{r}_\perp) \end{pmatrix} e^{ik_z z}. \tag{S42}$$

Inserting this into Eq.(S40), and after some algebra, we obtain the linear system

$$\begin{bmatrix} \xi v_z k_z - \lambda\epsilon_{n,\mathbf{k}} & \alpha_n(\hat{D}^\dagger)^n \\ \alpha_n(\hat{D})^n & -\xi v_z k_z - \lambda\epsilon_{n,\mathbf{k}} \end{bmatrix} \begin{pmatrix} F(\mathbf{r}_\perp) \\ G(\mathbf{r}_\perp) \end{pmatrix} = 0, \tag{S43}$$

where we have defined the differential operators [2] $\hat{D} = -i\partial_x + i(-i\partial_y)$ and $\hat{D}^\dagger = -i\partial_x - i(-i\partial_y)$. Using the fact that $\epsilon_{n,\mathbf{k}}^2 - v_z^2 k_z^2 = \alpha_n^2 k_\perp^2$, the system above can be reduced to

$$\left[(\hat{D}^\dagger)^n(\hat{D})^n - k_\perp^{2n}\right] F(\mathbf{r}_\perp) = 0 \tag{S44}$$

$$G(\mathbf{r}_\perp) = \frac{\alpha_n}{\xi v_z k_z + \lambda\epsilon_{n,\mathbf{k}}} (\hat{D})^n F(\mathbf{r}_\perp). \tag{S45}$$

We notice that, by definition, $\left[\hat{D}, \hat{D}^\dagger\right] = 0$, and $\hat{D}\hat{D}^\dagger = -\nabla_\perp^2$. Therefore, Eq.(S44) reduces to

$$\left[(-\nabla_\perp^2)^n - k_\perp^{2n}\right] F(\mathbf{r}_\perp) = 0. \tag{S46}$$

To find the general solutions to this differential equation, it is convenient to factorize the operator, by making use of the $n$ complex roots of $k_\perp^{2n}$, which can be parameterized as $k_\perp^2 e^{i2(l-1)\pi/n}$, for $1 \le l \le n$. Hence, Eq.(S46) can be expressed as

$$\prod_{l=1}^{n} \left[-\nabla_\perp^2 - e^{i2(l-1)\pi/n} k_\perp^2\right] F(\mathbf{r}_\perp) = 0. \tag{S47}$$

In order to find solutions for each angular momentum channel $M = m' + n/2$, we proceed to expand in polar coordinates $\mathbf{r}_\perp = (r\cos\phi, r\sin\phi)$,

$$F(\mathbf{r}_\perp) = \sum_{m'\in\mathbb{Z}} \sum_{l=1}^{n} c_M^{(l)} e^{i(M-n/2)\phi} f_M^{(l)}(r). \tag{S48}$$

Therefore, for each component $f_M^{(l)}(r)$, and for each independent factor in the operator, Eq. (S47) reduces to

$$\left[\frac{d^2}{dr^2}+\frac{1}{r}\frac{d}{dr}+e^{i2(l-1)\pi/n}k_\perp^2-\frac{(M-n/2)^2}{r^2}\right]f_M^{(l)}(r)=0. \tag{S49}$$

The general solution to this equation is a linear combination of Bessel functions of complex argument

$$f_M^{(l)}(r)=c_1^{(l)}J_{M-n/2}(e^{i(l-1)\pi/n}k_\perp r)+c_2^{(l)}Y_{M-n/2}(e^{i(l-1)\pi/n}k_\perp r). \tag{S50}$$

Furthermore, the normalizability implies that the wavefunctions have to be asymptotically bounded as $r\to\infty$ and only the solution with $l=1$ fulfills this property. Therefore, we have ($c_i^{(l)}=c_2^{(l)}=0$, $2\le l\le n$)

$$f_M(r)=c_1J_{M-n/2}(k_\perp r)+c_2Y_{M-n/2}(k_\perp r). \tag{S51}$$

Now, to obtain the second component of the spinor, we apply Eq. (S45),

$$\begin{aligned}G(\mathbf{r}_\perp)=&\frac{\alpha_n}{\xi v_zk_z+\lambda\epsilon_{n,\mathbf{k}}}\sum_{m'\in\mathbb{Z}}c_M(-i)^ne^{in\phi}\left(\partial_r+\frac{i}{r}\partial_\phi\right)^n\left(e^{i(M-n/2)\phi}f_M(r)\right)\\ =&\frac{\alpha_n}{\xi v_zk_z+\lambda\epsilon_{n,\mathbf{k}}}\sum_{m'\in\mathbb{Z}}c_M(-i)^ne^{i(M+n/2)\phi}\left(\partial_r-\frac{M-n/2}{r}\right)^nf_M(r).\end{aligned} \tag{S52}$$

By using the following operator identity, which can be readily proven by induction,

$$\left(\partial_x-\frac{\alpha}{x}\right)^nZ_\alpha(x)=(-1)^nZ_{\alpha+n}(x), \tag{S53}$$

for $Z_\alpha(x)\equiv\{J_\alpha(x),Y_\alpha(x)\}$, we then find from Eqs. (S52) and (S51) that the free-spinor for each angular momentum channel $M$ is given by

$$\Psi_{out,M}^{(\lambda,\xi)}(r,\phi,z)=e^{ik_zz}\begin{pmatrix}e^{i(M-n/2)\phi}\left(c_1J_{M-n/2}(k_\perp r)+c_2Y_{M-n/2}(k_\perp r)\right)\\ \frac{i^n\alpha_nk_\perp^n}{\xi v_zk_z+\lambda\epsilon_{n,\mathbf{k}}}e^{i(M+n/2)\phi}\left(c_1J_{M+n/2}(k_\perp r)+c_2Y_{M+n/2}(k_\perp r)\right)\end{pmatrix}. \tag{S54}$$

The asymptotic properties of the Bessel functions for $k_\perp r\gg1$

$$J_{M\pm\frac{n}{2}}(k_\perp r)\sim\sqrt{\frac{2}{\pi k_\perp r}}\cos\left(k_\perp r-(M\pm\frac{n}{2}+\frac{1}{2})\frac{\pi}{2}\right), \tag{S55}$$

$$Y_{M\pm\frac{n}{2}}(k_\perp r)\sim\sqrt{\frac{2}{\pi k_\perp r}}\sin\left(k_\perp r-(M\pm\frac{n}{2}+\frac{1}{2})\frac{\pi}{2}\right), \tag{S56}$$

then imply

$$\Psi_{out,M}^{(\lambda,\xi)}(r,\phi,z)\sim e^{ik_zz}\tilde{C}_M\sqrt{\frac{2}{\pi k_\perp r}}\begin{pmatrix}e^{i(M-n/2)\phi}\cos\left(k_\perp r-(M-\frac{n}{2}+\frac{1}{2})\frac{\pi}{2}+\delta_M\right)\\ \frac{i^n\alpha_nk_\perp^n}{\xi v_zk_z+\lambda\epsilon_{n,\mathbf{k}}}e^{i(M+n/2)\phi}\cos\left(k_\perp r-(M+\frac{n}{2}+\frac{1}{2})\frac{\pi}{2}+\delta_M\right)\end{pmatrix}. \tag{S57}$$

Here, we defined $\tilde{C}_M=\sqrt{c_1^2+c_2^2}$, and the phase shift $\tan\delta_M=-c_2/c_1$.

To determine the phase shift for every angular momentum channel, i.e. to explicitly obtain the form of $c_{1,2}$, we need to impose continuity of the spinor solution at the boundary of the dislocation region $r=a$,

$$\Psi_{out,M}^{(\lambda,\xi)}(r=a,\phi,z)=\Psi_{m,M}^{(\lambda,\xi)}(r=a,\phi,z), \tag{S58}$$

with $\Psi_{m,M}^{(\lambda,\xi)}(r=a,\phi,z)$ given by Eq. (S34). This condition leads to a linear system for the constants $c_1$ and $c_2$, which is straightforward to solve, leading to

$$\tan\delta_M=-\frac{c_2}{c_1}=\frac{J_{M-\frac{n}{2}}(k_\perp a)-\beta_MJ_{M+\frac{n}{2}}(k_\perp a)}{Y_{M-\frac{n}{2}}(k_\perp a)-\beta_MY_{M+\frac{n}{2}}(k_\perp a)}. \tag{S59}$$

Here, we have defined the coefficients

$$\beta_M=\left[\frac{(m-n)!}{m!}\right]^{1/2}\left(\frac{a}{\sqrt{2}l}\right)^n\left[\frac{L_{m-n}^{|M|+n/2}\left(\frac{a^2}{2l^2}\right)}{L_m^{|M|-n/2}\left(\frac{a^2}{2l^2}\right)}\right]. \tag{S60}$$

Now, let us apply the matching condition Eq. (S39), by choosing the case $k_z = 0$, and using the relation $M = m' + n/2$. By equating the coefficients of $e^{\pm ik_\perp r}$ on both sides, we obtain the system of equations

$$\begin{pmatrix} f_1(\phi) \\ f_2(\phi) \end{pmatrix} + \frac{1}{2\sqrt{\pi k_\perp}} \sum_{m'\in\mathbb{Z}} \begin{pmatrix} i^{m'} e^{i(m'\phi-(m'+1/2)\pi/2)} \\ \lambda i^{m'} e^{i(m'+n)\phi-(m'+1/2)\pi/2} \end{pmatrix} = \frac{1}{\sqrt{2\pi k_\perp}} \sum_{m'\in\mathbb{Z}} \tilde{C}_M \begin{pmatrix} e^{i(m'\phi-(m'+1/2)\pi/2+\delta_{m'})} \\ \lambda i^n e^{i((m'+n)\phi-(m'+n+1/2)\pi/2+\delta_{m'})} \end{pmatrix}, \tag{S61}$$

$$\sum_{m'\in\mathbb{Z}} \begin{pmatrix} i^{m'} e^{i(m'\phi+(m'+1/2)\pi/2)} \\ \lambda i^{m'} e^{i(m'+n)\phi+(m'+1/2)\pi/2} \end{pmatrix} = \sqrt{2} \sum_{m'\in\mathbb{Z}} \tilde{C}_M \begin{pmatrix} e^{i(m'\phi+(m'+1/2)\pi/2-\delta_{m'})} \\ \lambda i^n e^{i((m'+n)\phi+(m'+n+1/2)\pi/2-\delta_{m'})} \end{pmatrix}. \tag{S62}$$

This system leads to the solution for the constants

$$\tilde{C}_M = \frac{i^{M-n/2}}{\sqrt{2}} e^{i\delta_M}, \tag{S63}$$

as well as for the scattering amplitudes $f_{1,2}(\phi)$ in terms of the phase shifts (see also Eqs. (S59) and (S60))

$$\begin{pmatrix} f_1(\phi) \\ f_2(\phi) \end{pmatrix} = \frac{ie^{-i\frac{\pi}{4}}}{\sqrt{\pi k_\perp}} \sum_{m'\in\mathbb{Z}} e^{i\delta_M} \sin\delta_M \begin{pmatrix} e^{im'\phi} \\ \lambda e^{i(m'+n)\phi} \end{pmatrix}. \tag{S64}$$

The differential scattering cross-section, per unit length $L$, is given by the square modulus of the scattering amplitudes in Eq. (S64)

$$\begin{aligned} \frac{1}{L}\frac{d\sigma}{d\phi} = |f_1(\phi)|^2 + |f_2(\phi)|^2 = \frac{2}{\pi k_\perp} \sum_{m',m''\in\mathbb{Z}} e^{i(m'-m'')\phi} \sin\delta_{m'} \sin\delta_{m''} e^{i(\delta_{m'}-\delta_{m''})} \\ \equiv \frac{2}{\pi k_\perp} \sum_{m,m'\in\mathbb{Z}} F(\delta_m,\phi) F^*(\delta_{m'},\phi), \end{aligned} \tag{S65}$$

where $F(\delta_m, \phi) = \exp(i\delta_m + im\phi)\sin\delta_m$, as given by Eq. (12) of the main text. The total cross-section is thus obtained integrating over the scattering angle

$$\sigma(\epsilon_{n,\mathbf{k}}) = \int_0^L dz \int_0^{2\pi} d\phi \, \frac{1}{L}\frac{d\sigma}{d\phi} = \frac{4L\alpha_n^{1/n}}{\epsilon_{n,\mathbf{k}}^{1/n}} \sum_{m'=-\infty}^{+\infty} \sin^2\delta_M. \tag{S66}$$

## S3. TRANSMISSION AND LANDAUER CONDUCTANCE

Following a Landauer ballistic approach [2, 3], and assuming the dimensions of the sample are $L$ and $W$, we define the transmission function accross the dislocation from an effective cross-section in the $\phi$-direction

$$T_\xi(\epsilon_{n,\mathbf{k}},\phi) = \frac{1}{LW} \sum_{m,\lambda} \frac{L}{\sigma(E_m)} \frac{d\sigma}{d\phi} \delta\left(k_\perp - (\lambda E_m/\alpha_n)^{1/n}\right), \tag{S67}$$

where the $\delta$-function enforces the condition for elastic scattering. Assuming that the contacts are held at different chemical potentials, and possibly also different temperatures, such that their local distribution functions are given by Fermi-Dirac distributions $f_L(E)$ and $f_R(E)$, respectively, we have that the total current through the junction is given by the sum of the contributions from each of the Weyl nodes $\xi = \pm$, $I = I_+ + I_-$. The group velocity in the plane, for $\epsilon_{n,\mathbf{k}} = \alpha_n k_\perp^n$, is given by

$$v_\perp(\epsilon_{n,\mathbf{k}}) = \frac{\partial \epsilon_{n,\mathbf{k}}}{\partial k_\perp} = n\alpha_n^{1/n} \epsilon_{n,\mathbf{k}}^{1-1/n}, \tag{S68}$$

and hence the Landauer current arising from each node $\xi = \pm$ can be expressed by

$$I_\xi = LW \int_{-\infty}^{+\infty} dE \; v_\perp(E) \left[D_L(E) f_L(E) - D_R(E) f_R(E)\right] \bar{T}_\xi(E). \tag{S69}$$

Here, the density of states at each contact is $D_{L,R}(E)$, respectively, while the angle-averaged transmission function is given by $\bar{T}_\xi(E) = \int_{-\pi/2}^{\pi/2} d\phi \cos\phi\, T_\xi(E,\phi)$. Applying the identity

$$\int_{-\pi/2}^{\pi/2} d\phi\, \cos\phi\, e^{i(m'-m'')\phi} = \frac{2(-1)^2}{1-4p^2}\delta_{m'',m'+2p} + \frac{\pi}{2}\delta_{m',m''\pm 1}, \tag{S70}$$

we obtain (for $k_\perp = (E/\alpha_n)^{1/n}$):

$$\begin{aligned}\bar{T}_\xi(E) =& \frac{2Ln|E|^{1-2/n}\alpha_n^{2/n}}{\pi\sigma(E)} \sum_{m,\lambda} \delta\left(E - \lambda E_m\right) \qquad \text{(S71)}\\ &\times \left\{ \pi \sum_{m'\in\mathbb{Z}} \sin\delta_{m'} \sin\delta_{m'-1} \cos(\delta_{m'} - \delta_{m'-1}) + 2 \sum_{m',p\in\mathbb{Z}} \frac{(-1)^p}{1-4p^2} \sin\delta_{m'} \sin\delta_{m'-2p} \cos(\delta_{m'} - \delta_{m'-2p}) \right\}.\end{aligned}$$

On the other hand, assuming the contacts are semi-infinite, uniform and identical, the density of states at $k_z = 0$ at each of them is

$$D_L(E) = D_R(E) = \frac{4}{L}\sum_\lambda \int \frac{d^2k_\perp}{(2\pi)^2}\delta(E - \lambda\alpha_n k_\perp^n) = \frac{2|E|^{2/n-1}}{\pi L\, n\, \alpha_n^{2/n}} \tag{S72}$$

where the factor of 4 accounts for the two spin components and the two nodes, respectively.

By combining Eq.(S72), as well as Eq.(S72) and Eq.(S68) into Eq.(S69), we obtain an explicit expression for the current

$$I_\xi = \alpha_n^{1/n} \sum_{\lambda,m} \left[f_L(\lambda E_m) - f_R(\lambda E_m)\right] \mathcal{T}(\lambda E_m) \tag{S73}$$

where we have defined the effective transmission function

$$\mathcal{T}(E) = \mathcal{T}_0(E) \left\{ \frac{\pi}{2} \sum_{m'\in\mathbb{Z}} \sin\delta_{m'} \sin\delta_{m'-1} \cos(\delta_{m'} - \delta_{m'-1}) + \sum_{m',p\in\mathbb{Z}} \frac{(-1)^p}{1-4p^2} \sin\delta_{m'} \sin\delta_{m'-2p} \cos(\delta_{m'} - \delta_{m'-2p}) \right\} \tag{S74}$$

where

$$\mathcal{T}_0(E) = \frac{8Ln|E|^{1-1/n}}{\pi^2\sigma(E)} = \frac{2n|E|}{\pi^2\alpha_n^{1/n}\sum_M \sin^2\delta_M}, \tag{S75}$$

where we used the explicit form of $\sigma(E)$ given by Eq. (S66). This is the form of the transmission function used in Eq. (18) of the main text. Therefore, the effective transmission function, up to a prefactor, depends only on the effective flux carried by the dislocation and the monopole charge, which are both dimensionless.

Finally, assuming that both contacts are held at the same temperature $T_L = T_R = T$, but at different chemical potentials $\mu_L = \mu_R + eV$, the electrical conductance is obtained from Eq. (S73),

$$G(T,V) = \left.\frac{\partial I}{\partial V}\right|_T = \frac{\alpha_n^{1/n}}{T} \sum_{\lambda,\xi,m} \mathcal{T}(\lambda E_m) f_L(\lambda E_m)\left[1 - f_L(\lambda E_m)\right], \tag{S76}$$

where we applied the identity

$$\frac{\partial f_L(E)}{\partial V} = \frac{1}{T} f_L(E)\left[1 - f_L(E)\right]. \tag{S77}$$

This is the form of the conductance as given in Eq. (18) of the main text.

## S4. DIMENSIONLESS QUANTITIES

Here, we show that the phase shift $\delta_M$ in Eq. (S59) depends only on the effective flux, LL index and the the total angular momentum quantum number. To this end, we first notice that the combination $a/\ell$, with $\ell \sim 1/\sqrt{B_D}$ the magnetic length associated with the effective magnetic field $B_D$, entering the phase shift does not depend on the radius $a$. Indeed, $a/\ell = a\sqrt{B_D} \sim \sqrt{\Phi_D}$. Furthermore, using this result and Eq. (S13), the combination $k_\perp a$, with $k_\perp^n = E_m/\alpha_n$, can be readily shown to be $a$-independent:

$$k_\perp a = a\left(\frac{E_m}{\alpha_n}\right)^{1/n} \sim \frac{a}{\ell} \sim \sqrt{\Phi_D}. \tag{S78}$$

Finally, in the main text we use the following dimensionless quantities:

$$\tilde{E}_m = \frac{E_m}{\alpha_n(\hbar/a)^n} = \frac{\alpha_n\sqrt{(2qB\hbar)^n}}{\alpha_n(\hbar/a)^n}\sqrt{\frac{m!}{(m-n)!}} = (2N_\phi)^{n/2}\sqrt{\frac{m!}{(m-n)!}}, \tag{S79}$$

and

$$\tilde{I}_\xi = \frac{\hbar}{e\alpha_n(\hbar/a)^n} I_\xi. \tag{S80}$$

## S5. NORMALIZATION CONSTANTS

For the spinor eigenfunction presented in Eq. (S26), we define the normalization coefficients such that the full spinor is normalized to one,

$$\begin{aligned} 1 &= \int_0^L dz \int_0^\infty dr\, r \int_0^{2\pi} d\phi\, \Psi_{m,M}^{(\lambda,\xi)\dagger}(r,\phi,z)\Psi_{m,M}^{(\lambda,\xi)}(r,\phi,z) \\ &= L|\mathcal{C}|^2\left\{\left(1+\lambda\xi\frac{v_z k_z}{E_m}\right)A_+ + \left(1-\lambda\xi\frac{v_z k_z}{E_m}\right)A_-\right\}. \end{aligned} \tag{S81}$$

Here, we defined the coefficients

$$A_+ = \int_0^{2\pi}\int_0^\infty dr\, r\left|\psi_{m-n}^M(r,\phi)\right|^2 = 2\pi(m-n)!\int_0^\infty dr\, r\, e^{-\frac{r^2}{2\ell^2}}\left(\frac{r^2}{2\ell^2}\right)^{|M|+\frac{n}{2}}\left[L_{m-n}^{|M|+\frac{n}{2}}\left(\frac{r^2}{2\ell^2}\right)\right]^2 \tag{S82}$$

$$A_- = \int_0^{2\pi}\int_0^\infty dr\, r\left|\psi_m^M(r,\phi)\right|^2 = 2\pi m!\int_0^\infty dr\, r\, e^{-\frac{r^2}{2\ell^2}}\left(\frac{r^2}{2\ell^2}\right)^{|M|-\frac{n}{2}} = \left[L_m^{|M|-\frac{n}{2}}\left(\frac{r^2}{2\ell^2}\right)\right]^2 \tag{S83}$$

Let us introduce the change of variables $z = r^2/(2\ell^2)$, with $0 \le z < \infty$. Then, we have that both integrals can be calculated as

$$A_+ = 2\pi(m-n)!\ell^2\int_0^\infty dz\, e^{-z}z^{|M|+\frac{n}{2}}\left[L_{m-n}^{|M|+\frac{n}{2}}(z)\right]^2 = 2\pi\ell^2\left(|M|+m-\frac{n}{2}\right)! \tag{S84}$$

and

$$A_- = 2\pi m!\ell^2\int_0^\infty dz\, e^{-z}z^{|M|-\frac{n}{2}}\left[L_m^{|M|-\frac{n}{2}}(z)\right]^2 = 2\pi\ell^2\left(|M|+m-\frac{n}{2}\right)! \tag{S85}$$

Here, we used the identity

$$\int_0^\infty x^\alpha e^{-x}L_n^\alpha(x)L_m^\alpha(x) = \frac{(n+\alpha)!}{n!}\delta_{n,m} \tag{S86}$$

Upon substitution into Eq.(S81), we solve for the overall normalization constant,

$$\mathcal{C} = \frac{1}{\sqrt{4\pi L\ell^2\left(|M|+m-n/2\right)!}}. \tag{S87}$$

[1] I. S. Gradshteyn and I. M. Ryzhik, Table of integrals, series, and products (Academic press, 2014).
[2] E. Muñoz and R. Soto-Garrido, J. Phys.: Condens. Matter **29**, 445302 (2017).
[3] R. Soto-Garrido and E. Muñoz, J. Phys.: Condens. Matter **30**, 195302 (2018).
